# Supplementary material for: SIGNER: Temporally Grounded Sign Language Generation via Time-Resolved Conditioning
Source: arXiv:2506.07460 source file (2026-06-26)
Supplement: Supplementary file 1 [file suppl.tex]

\begin{table*}[t]
\footnotesize
\centering
\setlength\tabcolsep{4.2pt}

\resizebox{0.98\textwidth}{!}{
\begin{tabular}{
    >{\centering\arraybackslash}m{5cm}
    >{\centering\arraybackslash}m{2.8cm}
    >{\centering\arraybackslash}m{1.2cm}
    >{\centering\arraybackslash}m{2cm}
    >{\centering\arraybackslash}m{1.3cm}
    >{\centering\arraybackslash}m{0.35cm}
    >{\centering\arraybackslash}m{1.2cm}
    >{\centering\arraybackslash}m{1.4cm}
    >{\centering\arraybackslash}m{1.3cm}
}
\specialrule{.1em}{.05em}{.05em}
\multirow{2}{*}{\textbf{Used evaluator setting}}
& \multirow{2}{*}{\textbf{Method}}
& \multicolumn{3}{c}{\textbf{CSL-Daily}}
&& \multicolumn{3}{c}{\textbf{Phoenix-2014T}} \\
\cline{3-5} \cline{7-9}
& & WER$\downarrow$ & BLEU-4$\uparrow$ & ROUGE$\uparrow$
&& WER$\downarrow$ & BLEU-4$\uparrow$ & ROUGE$\uparrow$ \\
\specialrule{.15em}{.1em}{.1em}

\multirow{9}{*}{\textbf{Our evaluator}}
& GT (test set)              & 37.86 & 22.44 & 49.20 && 39.32 & 20.73 & 41.51 \\
\cline{2-9}
& MotionGPT~\cite{motiongpt} & 94.92 & 1.79  & 15.48 && 99.60 & 0.81  & 7.07 \\
& MDM~\cite{mdm}             & 95.54 & 2.78  & 16.29 && 99.83 & 0.97  & 7.40 \\
& NSA~\cite{nsa}             & 96.64 & 2.09  & 14.56 && 98.29 & 1.03  & 7.62 \\
& MoMask~\cite{momask}       & 91.51 & 3.79  & 20.12 && 92.01 & 5.15  & 22.80 \\
& SOKE~\cite{soke}           & 85.69 & 4.09  & 21.70 && 87.74 & 5.52  & 19.69 \\
& G2P-DDM~\cite{g2p-ddm}     & 74.28 & 6.44  & 25.31 && 88.00 & 5.17  & 16.78 \\
& NAT-EA~\cite{natat}        & 67.80 & 7.87  & 29.17 && 75.65 & 8.79  & 23.04 \\
& \textbf{Ours}              & \textbf{55.05} & \textbf{15.60} & \textbf{39.52}
                             && \textbf{67.16} & \textbf{11.46} & \textbf{29.39} \\
\hline
\hline

\multirow{9}{*}{\shortstack{\textbf{Previous}\\\textbf{skeleton-based}\\\textbf{evaluator}\\\textbf{(as in~\cite{g2p-ddm,natat})}}}
& GT (test set)              & 43.65 & 17.08 & 44.08 && 54.55 & 10.69 & 27.66 \\
\cline{2-9}
& MotionGPT~\cite{motiongpt} & 94.32 & 1.75 & 15.95 && 95.72 & 2.13 & 10.84 \\
& MDM~\cite{mdm}             & 92.16 & 2.41 & 16.94 && 91.21 & 3.40 & 15.61 \\
& NSA~\cite{nsa}             & 91.66 & 2.81 & 18.95 && 94.11 & 3.19 & 14.19 \\
& MoMask~\cite{momask}       & 89.78 & 3.44 & 20.65 && 82.01 & 7.15 & 20.80 \\
& SOKE~\cite{soke}           & 80.94 & 4.17 & 21.89 && 82.86 & 6.81 & 20.33 \\
& G2P-DDM~\cite{g2p-ddm}     & 75.01 & 5.96 & 25.37 && 79.66 & 7.87 & 20.65 \\
& NAT-EA~\cite{natat}        & 78.27 & 5.43 & 25.22 && 80.89 & 7.35 & 20.57 \\
& \textbf{Ours}              & \textbf{60.17} & \textbf{11.78} & \textbf{34.94}
                             && \textbf{72.54} & \textbf{8.76} & \textbf{23.67} \\
\hline
\hline

\multirow{3}{*}{\shortstack{\textbf{Originally reported score}\\\textbf{(using skeleton-based}\\\textbf{evaluator as in~\cite{g2p-ddm,natat})}}}
& GT (test set)              & \multicolumn{3}{c}{Not reported} && 55.93 & 10.58 & 27.70 \\
\cline{2-9}
& G2P-DDM~\cite{g2p-ddm}     & -- & -- & -- && 77.26 & 7.50 & -- \\
& NAT-EA~\cite{natat}        & -- & -- & -- && 82.01 & 6.66 & 19.43 \\
\specialrule{.1em}{.05em}{.05em}
\end{tabular}
}
\vspace{2mm}
\caption{\textbf{Comparison under different evaluator settings.}
We report back-translation results on CSL-Daily and Phoenix-2014T under three evaluator settings:
(1) our evaluator, (2) the previous skeleton-based evaluator, and (3) originally reported scores from prior works that use the previous evaluator.}
\vspace{-5mm}
\label{tab:fairness_eval}
\end{table*}

\section{Cross-evaluator evaluation}
Previous works evaluate linguistic metrics such as WER~\cite{wer}, BLEU~\cite{bleu}, and ROUGE~\cite{rouge} using different back-translation models, making direct comparison difficult.
In particular, the reported test-set performance of the ground-truth motion varies across papers, indicating that the evaluator itself differs across methods.
For example, NSA~\cite{nsa} and SOKE~\cite{soke} rely on their own back-translation models, which are not publicly available, while G2P-DDM~\cite{g2p-ddm} and NAT-EA~\cite{natat} use a skeleton-based evaluator.
Such inconsistency makes the reported linguistic scores not directly comparable across prior works.

Our method uses a motion representation that includes not only body and hand joints but also facial expressions.
Accordingly, evaluating our model with a skeleton-based back-translation model is suboptimal, as such an evaluator cannot fully assess the information preserved in face-aware motion sequences.
For a fair and expressive comparison, we therefore train a unified evaluator on the same face-inclusive motion representation used in our method, and apply this evaluation setup to all compared baselines.
Likewise, all comparison baselines are trained and evaluated using the same face-inclusive data representation, and generate motions with facial expressions as well (see the qualitative comparison videos in the supplementary material).

\noindent\textbf{Our evaluator.}
We train a unified sign-to-text back-translation model on the same motion representation used throughout our framework, which includes body, hand, and facial components.
Our evaluator is built by adapting the TwoStream framework~\cite{chen2022twostream} to our data format.
It consists of two stages: a recognition model that predicts a gloss sequence from the input motion, and a translation model that reconstructs the spoken-language text.

The recognition model is composed of a pose encoder and a prediction head.
For the pose encoder, we adopt an P3D-based~\cite{p3d} architecture.
Each frame of the input pose sequence is represented using 43 joints with three modalities: 3D joint coordinates (129 dimensions), 6D joint rotations (258 dimensions), and a 13-dimensional facial expression vector.
These three components are first linearly projected into separate embedding spaces, yielding 256-dimensional joint embeddings, 256-dimensional rotation embeddings, and 64-dimensional expression embeddings.
They are then processed by independent temporal convolution encoders, producing modality-specific temporal features of dimensions 224, 224, and 64, respectively.
Finally, these features are concatenated to obtain a 512-dimensional pose representation for each frame.
This representation is further refined by a visual head composed of a linear projection layer, masked batch normalization, ReLU activation, positional encoding, dropout with rate 0.1, a position-wise feed-forward layer, and layer normalization.

For the translation stage, we initialize the translation network with pretrained mBART~\cite{mbart}.
We use mBART-${\text{de}}$ for Phoenix-2014T and mBART-${\text{zh}}$ for CSL-Daily.
To further stabilize back-translation quality, we initialize the translation network weights from a pretrained gloss-to-text checkpoint.
The gloss embeddings are also initialized from pretrained mBART-based gloss embeddings.
The features produced by the pose encoder are mapped into the mBART input space via a VLMapper, and the mapped features are then fed into the translation network for text generation.

We train the evaluator using Adam with $\beta=(0.9, 0.998)$ and weight decay $0.001$ for 50,000 iterations with 32 mini batch size.
We use a learning rate of $1\times10^{-5}$ for the translation network and $1\times10^{-4}$ for the remaining modules.
Mixed-precision training is enabled with GradScaler.

\noindent\textbf{Cross-evaluator evaluation.}
To further ensure transparency, we additionally evaluate all methods using the previous skeleton-based evaluator adopted in prior works such as G2P-DDM~\cite{g2p-ddm} and NAT-EA~\cite{natat}.
We report these results in the second block of Table~\ref{tab:fairness_eval}.
In the third block, we also list the originally reported scores of G2P-DDM and NAT-EA under their original evaluation setting.
The reproduced scores remain reasonably close to the originally reported numbers, suggesting that our reproduction under the previous evaluator is reliable.
More importantly, our method consistently outperforms prior approaches across evaluator choices, showing that the observed performance gains do not depend on a specific evaluator design.
These results support that the advantage of our method comes from improved generation quality rather than from the choice of the back-translation model.

\begin{table}[t]
\footnotesize
\centering
\setlength\tabcolsep{7pt}

\begin{tabular}{
    >{\centering\arraybackslash}m{2.7cm}
    >{\centering\arraybackslash}m{2.5cm}
    >{\centering\arraybackslash}m{2.3cm}
}
\specialrule{.1em}{.05em}{.05em}
Method & semantic accuracy$\uparrow$ & Naturalness$\uparrow$ \\
\specialrule{.15em}{.1em}{.1em}
MoMask~\cite{momask}       & 2.55 & 2.99 \\
NAT-EA~\cite{natat}        & 3.39 & 3.57 \\
Spoken2Sign~\cite{spoken2sign} & 3.66 & 2.80 \\
\textbf{Ours}              & \textbf{4.69} & \textbf{4.77} \\
\specialrule{.1em}{.05em}{.05em}
\end{tabular}
\vspace{1mm}
\caption{\textbf{Human evaluation.}
Participants rated generated sign motions on semantic accuracy and naturalness using a 0--5 scale.
SIGNER achieves the highest score in both criteria.
}
\label{tab:human_eval}
\end{table}

\section{Human evaluation}
We conduct a human evaluation to assess the semantic accuracy and naturalness of generated sign motions.
A total of 23 participants evaluated 6 samples per method using a 0--5 scale.
semantic accuracy measures how well the generated signing matches the intended meaning, while naturalness measures motion realism and transition quality.
We compare SIGNER with representative baselines, including MoMask~\cite{momask}, NAT-EA~\cite{natat}, and Spoken2Sign~\cite{spoken2sign}.
As shown in Table~\ref{tab:human_eval}, SIGNER achieves the highest scores in both semantic accuracy and naturalness, supporting the improvements observed in quantitative results.
